# Supplementary material for: Think Rationally about What You See: Continuous Rationale Extraction for Relation Extraction
Source: arXiv:2305.03503 source file (2023-05-02)
Supplement: Supplementary file 1 [file 9_appendix.tex]

\section{Distribution of the Dataset}
\label{distribution}

For training and development, the top twelve languages based on the number of labeled examples are included. The average number of examples per language is 1784, with Serbian being the smallest (835). The dataset is split into training
(75\%), development (10\%), and $\alpha_{1}$ test set (15\%). This leaves us with 13 languages for our zero-shot test set (and $\alpha_{3}$). The remaining set of sources form our out-of-domain test set (and $\alpha_{2}$).  In total, X-FACT covers the following 25 languages (shown with their ISO 639-1 code for brevity): ar, az, bn, de, es, fa, fr, gu, hi, id, it, ka, mr, no, nl, pa, pl, pt, ro, ru, si, sr, sq, ta, tr. Table~\ref{tab:language} shows the number of claims and languages.

There are 7 possible labels for each claim in XFact and EFact: True, Mostly-True, Partly-True, Mostly False, False, Unverifiable and Other.  Table~\ref{distribution} shows the composition of training, development, and test sets of XFact and EFact, respecitvely.

\input{tables/distribution}

\input{tables/language}

\section{Graph-based Model}\label{Graph-based Model}
In this section, we describe the Kernel Graph Attention Network (KGAT) \cite{Liu2020KernelGA} and how to use it for claim Verification. KGAT creates an evidence graph for claim $c$ by extracting evidence sentences $D=\{e^{1},...,e^{p},...,e^{l}\}$, and then utilizes the evidence graph to predict the claim label $y$.

KGAT builds the evidence graph $G$ by making each claim-evidence pair a node and connecting all node pairs with edges, resulting in a fully connected evidence graph with $l$ nodes as: $N=\{n^{1},...,n^{p},...,n^{l}\}$.

KGAT combines multiple and single evidence reasoning scenarios to generate a probability $P(y|c,D)$ for predicting the claim label $y$. In a graph neural network, KGAT uses the graph attention operation~\cite{Velickovic2018GraphAN} and splits the prediction into two parts: (1) the label prediction in each node conditioned on the whole graph $P(y|n^{p},G)$; (2) the evidence selection probability $P(n^{p}|G)$:
\begin{equation}
   P(y \mid c, D)=\sum_{p=1}^{l} P\left(y \mid c, e^{p}, D\right) P\left(e^{p} \mid c, D\right) 
\end{equation}
or in the graph notation:
\begin{equation}
P(y \mid G)=\sum_{p=1}^{l} P\left(y \mid n^{p}, G\right) P\left(n^{p} \mid G\right).
\end{equation}

The joint reasoning probability $P(y|n^{p},G)$ calculates node label prediction with multiple evidence. The readout module \cite{knyazev2019understanding} calculates the probability $P(n^{p}|G)$ and attentively combines per-node signals for prediction.

\section{Limitations}
\label{limitation}

In this paper,  we propose incorporating full text of web pages returned by the search engine for verifying real-world claims. Though the proposed fact-checking system significantly outperforms baselines, it still has the following three major limitations. Firstly, the training corpus only contains claims selected and verified by fact-checkers, as it is crawled from fact-checking agencies. Fact-checkers select and verify claims based on their judgements as well as public interests. Thus, there is no guarantee that the training corpus can cover any topics. Secondly, evidence in the retrieved web pages can be exhibited in the tables, PDFs, images, audios and videos. Human fact-checkers are able to extract relevant information from these heterogeneous sources, while our fact-checking system can only extract textual sentences as evidence. Unlike an artificial fact-checking dataset that assumes the world knowledge is restricted to Wikipedia, real-world dataset requires knowledge from more diversified sources. Using a search engine is an effective approach to obtain related knowledge, but it also brings the concern of untrustworthy evidence. Not all web documents returned by the search engine are equally trustworthy, and sometimes trustworthy sources contradict each other. Almost all existing fact-checking systems including ours are not able to address the presence of disagreeing or untrustworthy evidence.
